# Supplementary material for: Sea-level projections representing deeply uncertain ice-sheet contributions
Source: arXiv:1609.07119 ancillary file (2016-09-22)
Supplement: Supplementary file 1 [file Bakker_etal_Supplements.pdf]

# SUPPLEMENTARY INFORMATION

## Sea-level projections accounting for deeply uncertain ice-sheet contributions

Alexander M.R. Bakker[1,2,*], Tony E. Wong[1], Kelsey L. Ruckert[1], and Klaus Keller[1,3,4]

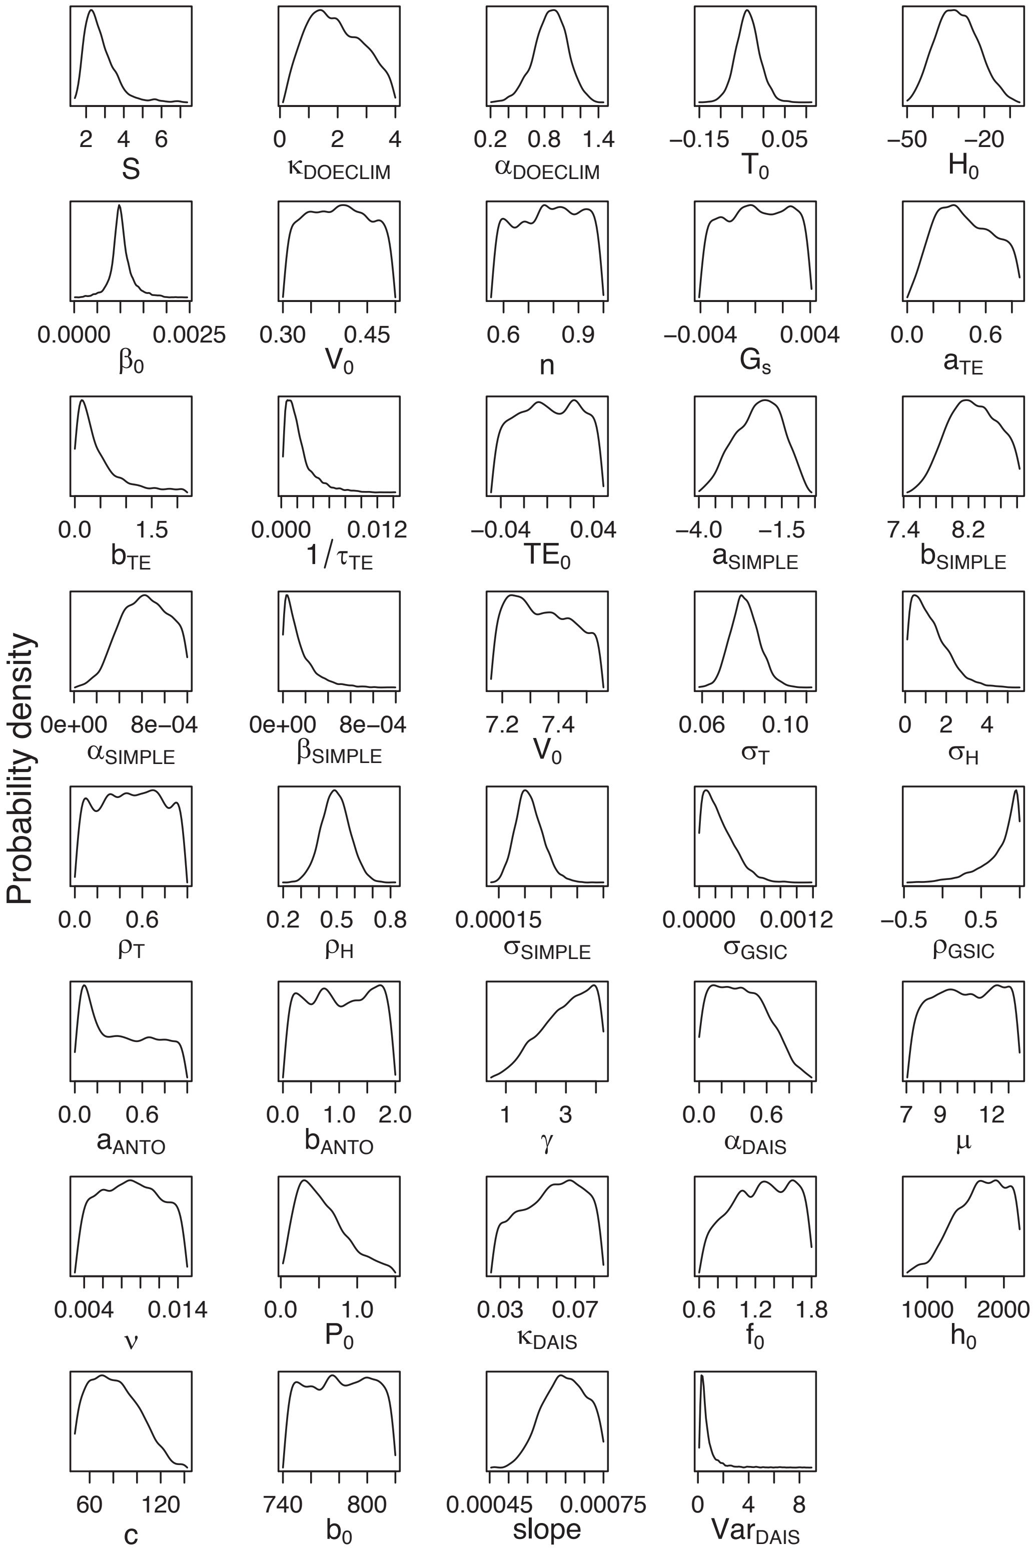


Figure S1 | Marginal posterior distributions of 39 free parameters.

| Contribution | Model | Data |
|---|---|---|
| Surface temperature | DOECLIM (Kriegler, 2005) | Morice et al., 2012 |
| Ocean heat uptake | DOECLIM (Kriegler, 2005) | Gouretski and Koltermann, 2007 |
| Glaciers and small ice caps | GSIC-MAGICC (Wigley and Raper, 2005) | Dyurgerov and Meier, 2005 |
| Thermal expansion | TE (Mengel et al., 2016) | Church et al., 2013 |
| Greenland ice sheet | SIMPLE (Bakker et al, 2016) | Sasgen et al., 2012 |
| Antarctic ice sheet | DAIS (Shaffer 2014) | Shaffer 2014; Ruckert et al., 2016; Church et al., 2013 |

Table S1 | Component models and calibration data used.

| Contribution | RCP2.6 | RCP4.5 | RCP8.5 |
|---|---|---|---|
| Thermal expansion | 13.3 (7.65-22.0) | 15.8 (8.24-27.4) | 19.9 (9.00-36.5) |
| Glaciers and small ice caps | 11.9 (8.34-16.5) | 14.0 (9.84-19.1) | 17.2 (12.3-22.9) |
| Greenland ice sheet | 18.1 (12.1-27.5) | 31.3 (20.2-47.2) | 66.1 (39.8-96.9) |
| Antarctic ice sheet | 8.73 (1.25-17.2) | 9.97 (1.79-19.4) | 12.8 (2.78-24.7) |
| Total | 52.6 (39.9-70.8) | 71.5 (53.9-97.1) | 116 (84.5-159) |

Table S2 | Sea-level contribution in 2100, relative to 1986-2005 mean sea level (cm SLE)

| Parameter | Model | Median | 5% quantile | 95% quantile | Lower bound | Upper bound | Units |
|---|---|---|---|---|---|---|---|
| S | DOECLIM | 2.552 | 1.787 | 4.317 | 0.1 | 10 | °C |
| $\kappa_{DOECLIM}$ | DOECLIM | 1.888 | 0.4791 | 3.656 | 0.1 | 4 | $cm^2 s^{-1}$ |
| $\alpha_{DOECLIM}$ | DOECLIM | 0.8759 | 0.553 | 1.158 | 0 | 2 | - |
| $T_0$ | DOECLIM | -0.03695 | -0.08114 | 0.01047 | -0.3 | 0.3 | °C |
| $H_0$ | DOECLIM | -30.89 | -43.15 | -16.72 | -50 | 0 | $10^{22}$ J |
| $\sigma_T$ | DOECLIM | 0.08029 | 0.06989 | 0.09215 | 0.05 | 5 | °C |
| $\sigma_H$ | DOECLIM | 1.054 | 0.1891 | 2.835 | 0.1 | 10 | $10^{22}$ J |
| $\rho_T$ | DOECLIM | 0.5005 | 0.04763 | 0.9465 | 0 | 0.999 | - |
| $\rho_H$ | DOECLIM | 0.4915 | 0.3657 | 0.6244 | 0 | 0.999 | - |
| $\beta_0$ | GSIC | 0.000997 | 0.00066 | 0.001464 | 0 | 0.041 | m $y^{-1}$ °$C^{-1}$ |
| $V_{0,GSIC}$ | GSIC | 0.3997 | 0.3103 | 0.4896 | 0.3 | 0.5 | m |
| n | GSIC | 0.78 | 0.5738 | 0.9773 | 0.55 | 1 | - |
| $G_{s,0}$ | GSIC | 4.45E-05 | -0.003625 | 0.003688 | -0.0041 | 0.0041 | m |
| $\sigma_{GSIC}$ | GSIC | 0.0002078 | 1.81E-05 | 0.0006155 | 0 | 0.0015 | m |
| $\rho_{GSIC}$ | GSIC | 0.8424 | 0.2056 | 0.9891 | -0.999 | 0.999 | - |
| $a_{TE}$ | TE | 0.4265 | 0.1051 | 0.8074 | 0 | 0.8595 | m °$C^{-1}$ |
| $b_{TE}$ | TE | 0.33 | 0.0337 | 1.728 | 0 | 2.193 | m |
| $1/\tau_{TE}$ | TE | 0.00172 | 0.0004294 | 0.005997 | 0 | 1 | $y^{-1}$ |
| $TE_0$ | TE | 0.0005103 | -0.04287 | 0.04339 | -0.0484 | 0.0484 | m |
| $a_{SIMPLE}$ | SIMPLE | -2.142 | -3.364 | -1.121 | -4 | -0.001 | m °$C^{-1}$ |
| $b_{SIMPLE}$ | SIMPLE | 8.255 | 7.766 | 8.745 | 5.888 | 8.832 | m |
| $\alpha_{SIMPLE}$ | SIMPLE | 0.0006293 | 0.0002762 | 0.0009549 | 0 | 0.001 | $y^{-1}$ °$C^{-1}$ |
| $\beta_{SIMPLE}$ | SIMPLE | 0.0001002 | 7.71E-06 | 0.0004376 | 0 | 0.001 | $y^{-1}$ |
| $V_{0,SIMPLE}$ | SIMPLE | 7.347 | 7.178 | 7.54 | 7.16 | 7.56 | m |
| $\sigma_{SIMPLE}$ | SIMPLE | 0.0002067 | 0.0001697 | 0.0002544 | 0 | 0.002 | m |
| $\rho_{SIMPLE}$ | SIMPLE | 0.8821 | 0.8821 | 0.8821 | 0.8821 | 0.8821 | - |
| $a_{ANTO}$ | ANTO | 0.4399 | 0.03937 | 0.9479 | 0 | 1 | °C °$C^{-1}$ |
| $b_{ANTO}$ | ANTO | 1.005 | 0.1052 | 1.896 | 0 | 2 | °C |
| $\gamma$ | DAIS | 3.113 | 1.391 | 4.146 | 0.5 | 4.25 | - |
| $\alpha_{DAIS}$ | DAIS | 0.3611 | 0.03808 | 0.7807 | 0 | 1 | - |
| $\mu$ | DAIS | 10.46 | 7.432 | 13.38 | 7.05 | 13.65 | $m^{1/2}$ |
| $\nu$ | DAIS | 0.008997 | 0.003788 | 0.01429 | 0.003 | 0.015 | $m^{-1/2} y^{-1/2}$ |
| $P_0$ | DAIS | 0.5062 | 0.1276 | 1.253 | 0.026 | 1.5 | m $y^{-1}$ |
| $\kappa_{DAIS}$ | DAIS | 0.05742 | 0.02845 | 0.08192 | 0.025 | 0.085 | °$C^{-1}$ |
| $f_0$ | DAIS | 1.264 | 0.6927 | 1.744 | 0.6 | 1.8 | m $y^{-1}$ |
| $h_0$ | DAIS | 1718 | 1094 | 2161 | 735.5 | 2206.5 | m |
| c | DAIS | 80.05 | 51.2 | 120.9 | 47.5 | 142.5 | m °$C^{-1}$ |
| $b_0$ | DAIS | 780.4 | 744.3 | 816.6 | 740 | 820 | m |
| slope | DAIS | 0.0006488 | 0.0005511 | 0.0007352 | 0.00045 | 0.0007 | - |
| $Var_{DAIS}$ | DAIS | 0.5067 | 0.1887 | 2.262 | 0 | 2 | $m^2$ |

Table S3 | Parameters, units, models, prior ranges, and posterior distribution statistics.

| Study | DOECLIM | MAGICC | SIMPLE | DAIS-ANTO | TE |
|---|---|---|---|---|---|
| Urban & Keller (2010) | X | | | | |
| Wigley & Raper (2005) | | X | | | |
| Church et al (2001) | | X | | | |
| Chen & Ohmura (1990) | | X | | | |
| Marčelja (2010), | | | | | X |
| Mengel et al (2016) | | | | | X |
| Church & White (2011) | | X | X | X | X |
| Bakker et al (2016) | | | X | | |
| Ridley et al (2010) | | | X | | |
| Bamber et al (2013) | | | X | | |
| Applegate et al (2012) | | | X | | |
| Robinson et al (2012) | | | X | | |
| Shaffer (2014) | | | | X | |
| Oerlemans (2005) | | | | X | |
| Oerlemans (2003) | | | | X | |
| Ruckert et al (2016) | | | | X | |
| Kotlyakov (1966) | | | | X | |
| Bryazgin (1986) | | | | X | |
| Pollard & DeConto (2009) | | | | X | |
| Thadathil et al (2002) | | | | X | |

Table S4 | Literature used to formulate prior probability density functions for the calibration

**References**


Applegate, P. J. *et al.* An assessment of key model parametric uncertainties in projections of Greenland Ice Sheet behavior. *The Cryosphere* 6, 589-606 (2012)

Bakker, A. M. R., Applegate, P. J. & Keller, K. A simple, physically motivated model of sea-level contributions from the Greenland ice sheet in response to temperature changes. *Environmental Modelling & Software* 83, 27-35 (2016)

Bamber *et al* A new bed elevation dataset for Greenland. *The Cryosphere* 7, 499-510 (2013).

Bryazgin (1986, "Method of preparing monthly charts of atmospheric precipitation in Antarctica")

Chen and Ohmura (1990, "Estimation of Alpine glacier water resources and their change since the 1870s")

Church, J. A. & White, N. J. Sea-level rise from the late 19th to the early 21st century. *Surveys in Geophysics* 32, 585–602 (2011).

Church, J. A. *et al.* Sea level change. In Stocker, T. F. et al. (eds.) *Climate Change 2013: The Physical Science Basis. Contribution of Working Group I to the Fifth Assessment Report of the Intergovernmental Panel on Climate Change*, 1137–1216 (Cambridge University Press, Cambridge, United Kingdom and New York, NY, USA, 2013).

Dyurgerov, M. B. & Meier, M. F. *Glaciers and the changing Earth system: a 2004 snapshot*. 58, (Institute of Arctic and Alpine Research, University of Colorado Boulder, 2005)

Gouretski, V. & Koltermann, K. P. How much is the ocean really warming? *Geophysical Research Letters* 34 (2007)

Kotlyakov (1966, "The snow cover of the Antarctic and its role in the present-day glaciation of the continent")

Kriegler, E. *Imprecise Probability Analysis for Integrated Assessment of Climate Change*. Ph.D. thesis, Universität Potsdam, Potsdam (2005). URL https://www.pik-potsdam.de/members/edenh/theses/PhDKriegler.pdf

Marčelja, S. The timescale and extent of thermal expansion of the global ocean due to climate change. *Ocean Science* 6, 179-184 (2010).

Mengel, M. *et al.* Future sea level rise constrained by observations and long-term commitment. *Proceedings of the National Academy of Sciences of the United States of America (PNAS)* 113, 2597–2602 (2016).Morice et al. (2012)

Oerlemans, J. Antarctic ice volume for the last 740 ka calculated with a simple ice sheet model. *Antarctic Science* 17, 281-287 (2005)

Oerlemans, J. A quasi-analytical ice-sheet model for climate studies. *Nonlinear processes in geophysics* 10, 441-452 (2003)

Pollard, D. & DeConto, R. M. Modelling West Antarctic ice sheet growth and collapse through the past five million years. *Nature* 458, 329-332 (2009)

Ridley, J. *et al.* Thresholds for irreversible decline of the Greenland ice sheet. *Climate Dynamics* 35, 1049-1057 (2010)

Robinson, A. *et al.* Multistability and critical thresholds of the Greenland ice sheet. *Nature Climate Change* 2, 429-432 (2012)

Ruckert, K. L., Shaffer, G., Pollard, D., Guan, Y., Wong, T.E., Forest, C. E. & Keller, K. The neglect of cliff instability can underestimate warming period melting in Antarctic ice sheet model, (2016) Neglecting cliff instability in Antarctic ice sheet models can reduce melting during warming periods. *arXiv:1609.06338* (2016).

Sasgen *et al.* Timing and origin of recent regional ice-mass loss in Greenland. *Earth and Planetary Science Letters* 333/334, 293-303 (2012).

Shaffer, G. Formulation, calibration and validation of the dais model (version 1), a simple antarctic ice sheet model sensitive to variations of sea level and ocean subsurface temperature. *Geoscientific Model Development* 7, 1803–1818 (2014).

Thadathil et al (2002, doi:10.1175/1520-0426-19.3.391).Ruckert, K. L., Shaffer, G., Pollard, D., Forest, C. E. & Keller, K. Neglecting cliff instability in Antarctic ice sheet models can reduce melting during warming periods. *PLoS ONE* (2016). In preparation.

Urban, N. M. & Keller, K. Probabilistic hindcasts and projections of the coupled climate, carbon cycle and Atlantic meridional overturning circulation system: a bayesian fusion of century-scale observations with a simple model. *Tellus* A 62, 737–750 (2010).

Wigley, T. M. L. & Raper, S. C. B. Extended scenarios for glacier melt due to anthropogenic forcing. *Geophysical Research Letters* 32 (2005)
